# Supplementary material for: MESH -- Understanding Videos Like Human: Measuring Hallucinations in Large Video Models
Source: arXiv:2509.08538 source file (2025-09-11)
Supplement: Supplementary file 1 [file appendix_empty.tex]

\appendix
\onecolumn
\section{Human understanding videos}\label{ap:human-under}

\section{MESH Benchmark}\label{ap:bench}
% \subsection{Dataset annotations}
% \subsubsection{Generating character features}\label{ap:mesh-char}

\subsection{Metric}
\subsubsection{Why using multi-choice questions?}\label{ap:metric-mc}

\subsubsection{Additional metric: JSD}\label{ap:metric-jsd}
% We present the calculation of \textit{Option Balance} (OB) and \textit{Correct Option Balance} (COB) metrics here. 
% \begin{align}
%     \text{OB} = \sqrt{ \frac{1}{4} \sum_{i=1}^{4} \left( P_i - \overline{P} \right)^2 }\\
%     \text{COB} = \sqrt{ \frac{1}{4} \sum_{i=1}^{4} \left( P_i^+ - \overline{P}^+ \right)^2 }
% \end{align}
% where $P_i = \frac{N_i}{N}$, $P_i^+ = \frac{N_i^+}{N^+}$, $N_i$ is the number of times option $i$ was selected, $N$ is the total number of questions, $N_i^+$ is the number of correct answers for option $i$, and $N^+$ is the total correct answers. 
% Models with lower OB and COB values produce a more balanced prediction distribution across the four MC question options. 
% In the following detailed results, we further employ Jensen-Shannon Divergence (JSD) \cite{jsd} to measure the option distribution between ground-truth and prediction. We have
% \[
% \text{JS}(P \| Q) = \frac{1}{2} \sum_{x} P(x) \ln \frac{P(x)}{M(x)} + \frac{1}{2} \sum_{x} Q(x) \ln \frac{Q(x)}{M(x)},
% \]
% where \( M(x) = \frac{1}{2}(P(x) + Q(x)) \). 
% % $P(x)$ and $Q(x)$ is the ground-truth and prediction distribution on "yes`` or "no`` choices in binary task and A/B/C/D choices in MC tasks.
% Here, \( P(x) \) represents the ground-truth distribution, and \( Q(x) \) represents the predicted distribution. For binary tasks, \( x \in \{\text{"yes"}, \text{"no"}\}\), while for multiple-choice tasks, \( x \in \{\text{A}, \text{B}, \text{C}, \text{D}\} \).We normalize the JSD for the binary task by dividing by 0.216 and for the MC task by dividing by 0.38.
% % \add{explaination of JSD}

\subsection{Setting hallucination}

\subsubsection{Uniqueness of Setting}\label{ap:mesh-hallu-set-uniq}

\subsubsection{Object Annotation}

\subsubsection{Selecting Setting}\label{ap:mesh-hallu-set-anno}

\subsection{Character hallucination}

\subsubsection{Uniqueness of Character}\label{ap:mesh-hallu-char-uniq}

\subsubsection{Generating character features}\label{ap:mesh-char}

\subsubsection{Selecting Character}\label{ap:mesh-hallu-char-anno}

\subsection{Stage hallucination}

\subsubsection{Uniqueness of Stage}\label{ap:mesh-hallu-stage-uniq}

\subsubsection{Filtering dialogue details}

\subsubsection{Annotated dialogues}\label{ap:mesh-dia}
% Conversation extraction is performed by analyzing TVQA+ subtitle talking information to identify conversational exchanges. Initially, the speaker's identity and temporal metadata (start/end timestamps) are extracted from the raw subtitle material. Subsequently, speaker names are systematically substituted with their corresponding feature descriptors (e.g., ``woman in a red blouse", ``man with glasses") using a predefined feature database derived from the person feature dataset. This process ensures anonymization while preserving contextual relevance through attribute-based identification. As illustrated in Figure 5a, this method produces anonymous output, such as ``A woman in a red dress without glasses is talking”, showing how the conversation is extracted from the video clip.

\subsubsection{Annotated actions}\label{ap:mesh-act}
% Action extraction is conducted using the TVQA+ question dataset and action timestamp annotations, with DeepSeek-v3 \cite{deepseekv3} facilitating the identification and refinement of non-conversational actions. To isolate purely physical interactions, questions addressing explanations, emotional states, or verbal exchanges are systematically filtered out through DeepSeek-v3 \cite{deepseekv3}. The retained question-answer pairs are then parsed to extract actions in the syntactic template “A does B,” where A represents the agent performing the action and B denotes the target entity (e.g., a person, object, or spatial context). Names within these extracted actions are substituted with their corresponding feature descriptors (e.g., garment type, gender) derived from the pre-extracted person feature database. Finally, the actions are temporally anchored to their respective video segments using the provided timestamp annotations. For instance, in the video clip illustrated in Figure 5b, the extracted action ``A man in a blue jacket without glasses is walking into the room” is generated through this process.

\subsubsection{Selecting Stage}\label{ap:mesh-hallu-stage-anno}

\subsection{Generalization of MESH annotation}\label{ap:transfer-method}

\section{Experiments}\label{ap:ep}
\subsection{General details}\label{ap:ep-gd}
\subsubsection{Difficulty level}\label{ap:ep-diff}

\subsubsection{Evaluated Video-Language Models}

\subsubsection{Technique Details}

% \paragraph{Deployment of Larger LVLMs with 8×A800 GPUs}

% For LVLMs exceeding 70 billion parameters—such as LLaVA-Video-72B, InternVL2.5-78B, Qwen2VL-72B, and LLaVA-OneVision-72B—we employ a high-performance computing node equipped with 8 NVIDIA A800 GPUs. To optimize inference speed, different deployment frameworks are utilized based on official recommendations and support. Specifically, LLaVA-OneVision-72B and Qwen2VL-72B, which provide official support for vLLM~\cite{vllm}, are deployed and evaluated using this framework. InternVL2.5-78B is deployed using the lmdeploy \cite{lmdeploy} framework, as recommended by its developers. For LLaVA-Video-72B, since it has not yet been integrated into other frameworks, we utilize the Hugging Face Transformers library \cite{huggingface} for deployment and evaluation.

% \paragraph{Deployment of Smaller LVLMs with RTX 3090/4090 GPUs}

% For LVLMs with fewer than 40 billion parameters—such as VILA1.5-8B, Aria-23B, and LLaVA-NeXT-Video-32B—the Hugging Face Transformers library is employed for model deployment and experimentation. To minimize computational costs, these models are deployed on consumer-grade GPUs, specifically the NVIDIA RTX 3090 and RTX 4090.

\subsection{Setting hallucination}\label{ap:ep-set}
\subsection{Character hallucination}\label{ap:ep-char}

\subsection{Stage hallucination}\label{ap:ep-sta}
\section{Additional Tables}\label{ap:tbs}

\section{Additional Case Study}\label{ap:case-study}

% \begin{figure}[h]
%     \centering
%     \includegraphics[width=1.0\columnwidth]{fig/CaseStudy1.pdf} % Adjust width to fit the entire column width
%     \caption{An example of one video and part of its corresponding hallucination questions.}
%     \label{fig:CaseStudy1}
% \end{figure}

% \begin{figure}[h]
%     \centering
%     \includegraphics[width=0.9\columnwidth]{fig/CaseStudy2.pdf} % Adjust width to fit the entire column width
%     \caption{Analysis of video question answering and description tasks reveals that LVMs exhibit a tendency to avoid generating descriptions for content that elicits uncertainty, as specifically detected through question answering; instances of hallucinated content are highlighted in red.}
%     \label{fig:CaseStudy2}
% \end{figure}
